# Supplementary material for: Warp and Learn: Novel Views Generation for Vehicles and Other Objects
Source: arXiv:1907.10634 source file (2020-10-10)
Supplement: Supplementary file 1 [file suppl_pascal_aug.tex]

\begin{figure}[tbh]
    \centering
    \includegraphics[width=0.95\columnwidth]{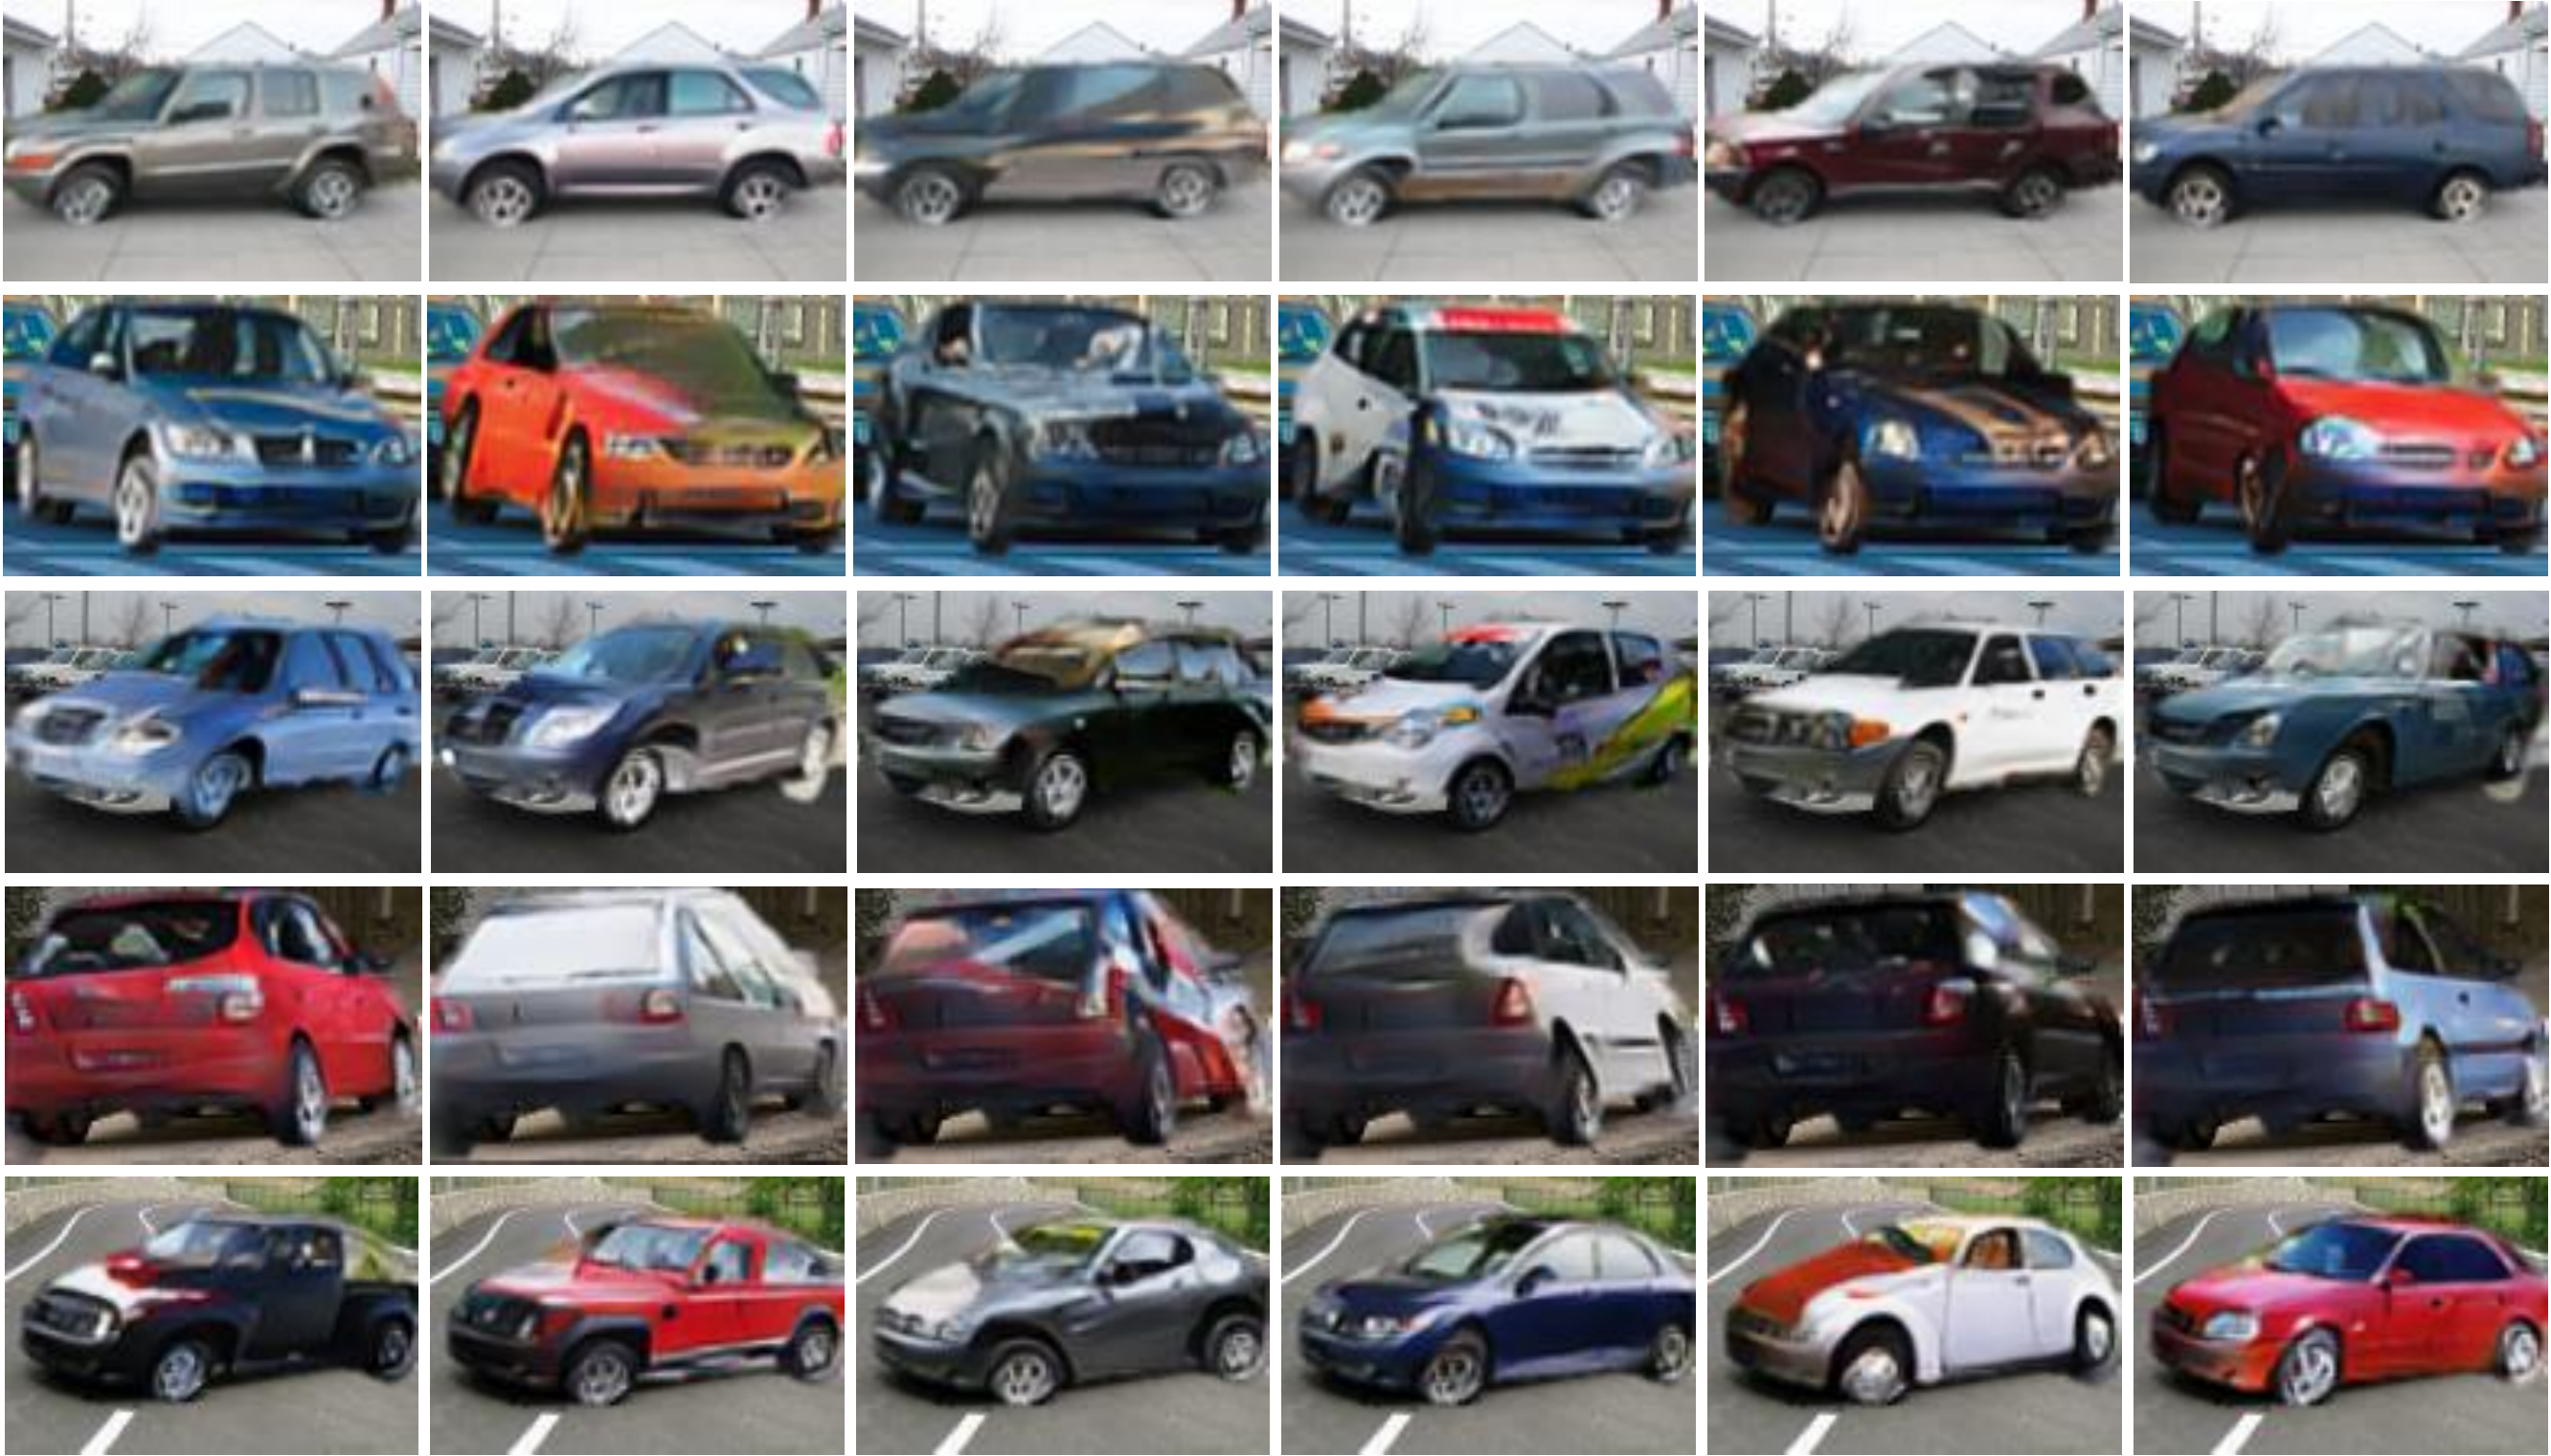}
    \caption{Examples of additional data generated stitching generated vehicles onto \pascal backgrounds.}
    \label{fig:suppl:pascal_aug}
\end{figure}
